# Supplementary material for: LEO Satellite Networking Relaunched: Survey and Current Research Challenges
Source: arXiv:2310.07646 source file (2023-10-11)
Supplement: Supplementary file 1 [file appendix.tex]

\allowdisplaybreaks
\section{TBD}
\label{app:basic-estimation}
